# Supplementary material for: Cross-Domain Ensemble Distillation for Domain Generalization
Source: arXiv:2211.14058 source file (2022-11-25)
Supplement: Supplementary file 3 [file _2_paper_correction.tex]

\section{Typo correction for Table.9 of our main paper}
\label{sec:supple_type_correction}
Before diving into additional results of our paper, we sincerely apologize for our typo in table 9 of our main paper. Even though we adopted the 40-2 Wide ResNet~\cite{zagoruyko2016wide} as the backbone network for the results of table 9 in our main paper, we wrote it wrong as WRN-28-10. Again, we are respectfully sorry for the typo, and remark that the experiment of table 9 in our main paper is conducted using the same backbone architecture (\ie, WRN-40-2) for a fair comparison, exactly following the protocol~\cite{hendrycks2019benchmarking,hendrycks2019augmix} to measure generalization to unseen corruptions.

%we exactly follow the protocol to measure generalization to unseen corruptions using \emph{the same backbone architecture} for a fair comparison, which is provided by \cite{hendrycks2019benchmarking}.
